# Supplementary material for: Revealing the topology of quasicrystals with a diffraction experiment
Source: arXiv:1607.00901 ancillary file (2017-11-23)
Supplement: Supplementary file 1 [file SuppMatPRLv5_resub.pdf]

# Supplemental Material for
# Revealing the topology of quasicrystals with a diffraction experiment

The supplementary material is organized as follows. In Section S1, we provide further information on the experimental methods used in the main article. In Section S2, we calculate the diffraction amplitudes for several patterns considered in the main article. In Section S3, we justify the claim from the main text about the linearity of the diffraction phase with the phason $\Phi$. In Section S4, we discuss the structural origin of topological numbers in Fibonacci chains, and show how the measured topological map arises naturally in a dual description of the $(x, \Phi)$ pattern studied in the experiment. Finally, in section S5, we report complementary measurements about the influence of noise on the diffraction pattern.

## S1-OPTICAL SETUP

We use a 532 nm laser source to illuminate our Digital Micromirror Device (DMD). The laser output is coupled into an optical fiber used as a spatial mode filter. The fiber output was expanded to obtain a Gaussian beam with $1/e^2$ radius of about 5 mm, apertured to give a roughly uniform illumination spot with a diameter of about 2.5 mm. This size was chosen empirically to obtain the sharpest observable diffraction peaks. For larger beams the imperfections (in particular, lack of flatness) of the DMD surface become more important and limit the achievable spot sizes.

The DMD (model DLP7000 from *Texas Instruments*) consists of a matrix of $1024 \times 768$ square micromirrors with a size $a = 14\,\mu$m. The angle of incidence of the laser on the DMD surface is on the order of 22° (see Fig. 1). Depending on the mirror state the light is reflected almost perpendicularly to the DMD plane (state B) or to a large angle and then blocked (state A). The diffracted light is focused on a CCD camera using a 2″ diameter aspherical lens with a focal of $f = 100$ mm. The axes of the CCD camera – corresponding to the reciprocal space from the DMD plane – are calibrated by imprinting a periodic lattice of period $2a$ on the DMD, which gives peaks separated from the zeroth order by $k_x = \pi/a$.

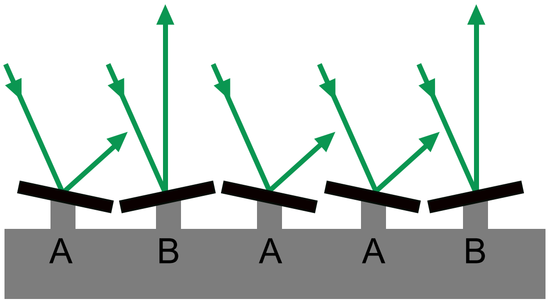


FIG. 1. Sketch of the DMD. Each mirror can be flipped individually between two positions. In position B light is reflected perpendicularly to the DMD surface and focused on the camera. In position A light is reflected with a larger angle and then blocked far away from the diffraction structure.

## S2-DIFFRACTION AMPLITUDES

We detail here the calculations of the diffraction patterns for various configurations studied in the main text. The Fibonacci chain of length $F_N$ is defined by $S_N(\Phi) \equiv [\chi_1\chi_2 \cdots \chi_{F_N}]$ with the characteristic function

$$\chi_n(\Phi) = \text{sign}\,\left[\cos\left(2\pi\, n\, \tau^{-1} + \Phi + \Phi_0\right) - \cos\left(\pi\, \tau^{-1}\right)\right]. \tag{1}$$

As in the main article, we choose $\Phi_0 = -(F_N + 1)\pi/\tau$, such that $\Phi = 0$ corresponds to a *palindromic* chain (*i.e.* $S_N = \overline{S}_N$ with $\overline{S}_N \equiv [\chi_{F_N} \cdots \chi_1]$) [1]. The reflectance $R_n$ of a vertical line of pixels at position $x = na$ is given by $R_n(\Phi) = \frac{1-\chi_n(\Phi)}{2}$ which is either 0 ( pixels $A$) or 1 (pixels $B$). The diffracted amplitude is thus proportional to the sum of phase factors over all the $B$ pixels, namely $\sum_B e^{ik_x x_B(\Phi)}$.

We first consider a single chain $S_N(\Phi)$ and a specific wavevector $k_q$ corresponding to one of the peaks of the diffraction pattern. The complex valued amplitude at this wavevector $k_q$ reads

$$A_q^{S_N}(\Phi) = \sum_B e^{ik_q x_B(\Phi)} \equiv \mathcal{A}_q^{S_N} e^{i\theta_q(\Phi)} \tag{2}$$

where $\mathcal{A}_q^{S_N}$ and $\theta_q(\Phi)$ are real numbers. The inverted structure $\overline{S}_N$ is obtained by replacing $x$ by $-x + aF_N$ ($a$ being the pixel size). We thus obtain the corresponding diffraction amplitude as

$$A_q^{\overline{S}_N}(\Phi) = \sum_B e^{ik_q(aF_N - x_B(\Phi))} = \mathcal{A}_q^{S_N} e^{-i\theta_q(\Phi)} e^{ik_q aF_N}. \tag{3}$$

We now take advantage of two results. First, the diffraction intensities at $k = k_q$ for the two structures $S_N$ and $\overline{S}_N$ are the same, and are independent of $\Phi$, $|A_q^{S_N}(\Phi)|^2 = |A_q^{\overline{S}_N}(\Phi)|^2 = (\mathcal{A}_q^{S_N})^2$. Second we note that, for a palindromic chain, the diffraction amplitudes are the same and hence we have $A_q^{S_N}(0) = A_q^{\overline{S}_N}(0)$ leading to $k_q aF_N = 2\theta_q(0)$.

We now proceed to describe the experiment "$S_N + S_N$". Defining the spatial origin at the center, we obtain

$$A_q^{S_N+S_N}(\Phi) = \mathcal{A}_q^{S_N} e^{i\theta_q(\Phi)}(e^{-2i\theta_q(0)} + 1). \tag{4}$$

As in the case of single chains, the diffraction intensities are identical for the structure and its reverse "$\overline{S}_N + \overline{S}_N$",

and independent of $\Phi$: $|A_q^{S_N+S_N}(\Phi)|^2 = 2(\mathcal{A}_q^{S_N})^2(1+\cos(2\theta_q(0)))$.

Finally, we consider the experiment "$S_N + \overline{S}_N$". We obtain

$$A_q^{S_N+\overline{S}_N}(\Phi) = \mathcal{A}_q^{S_N}\left(e^{i[\theta_q(\Phi)-2\theta_q(0)]} + e^{-i[\theta_q(\Phi)-2\theta_q(0)]}\right). \quad (5)$$

Unlike Eq. (4), the diffraction intensity $2(\mathcal{A}_q^{S_N})^2(1+\cos(2\theta_q(\Phi)-4\theta_q(0)))$ depends sinusoidally on $\theta_q(\Phi)$. In the next section we show that $\theta_q(\Phi)$ is a linear function of $\Phi$. The diffraction intensity then depends sinusoidally on $\Phi$ as observed experimentally.

## S3-THE PHASE TERM $\theta_q(\Phi)$

Here, we wish to show that the phase term $\theta_q(\Phi)$ in the diffraction amplitude of Eq. (2) is linear with $\Phi$, with a slope equal to the topological number $q$. A thorough proof will be given elsewhere [2]. Figure 2 shows how the phase $\theta_q(\Phi)$ of the diffraction amplitude varies as a function of $\Phi$ for different values of the wavevector $k_q$. The total diffraction phase $\theta_q(\Phi)$ is a staircase following a linear function of $\Phi$ with a slope $q$. Two more features are worth noting:

1. For a given value of $q$ (i.e. of $k_q$), the phases of $S_N$ and $\overline{S}_N$ are deduced from each other by changing $\Phi$ into $-\Phi$ (see Fig. 2).

2. Changing $k_q$ into $k_{-q}$ is equivalent to changing $\Phi$ into $-\Phi$.

These results seem to be a rather general feature of the diffraction pattern of both periodic and quasiperiodic structures (see for instance, for a generic discussion not restricted to 1D, [3–5]).

This linear dependence can be understood from a simple calculation. From the characteristic function $\chi_n$ in Eq. (1), we note that changing $\Phi$ from an initial value $\Phi_i$ by an amount $\Delta\Phi$ is equivalent to a spatial translation along the chain. Specifically, for $\Delta\Phi = 2\pi/\tau$, the resultant structure is translated by one pixel, and therefore the diffraction amplitude $A_q^{S_N}(\Phi_i + 2\pi/\tau)$ carries an additional phase, $\theta_q(\Phi_i + 2\pi/\tau) = \theta_q(\Phi_i) + ak_q$. Using the approximation $k_q = (2\pi/a)(p + q\tau^{-1})$, leads to $\theta_q(\Phi_i + 2\pi/\tau) = \theta_q(\Phi_i) + 2\pi q\tau^{-1} = \theta_q(\Phi_i) + q\Delta\Phi$. As a variation of $\Phi$ by $2\pi$ corresponds to $F_N$ structural changes (see Fig. 3c), then the shift $\Delta\Phi = 2\pi/\tau$ is associated with $F_N/\tau$ structural changes. Since each structural change amounts to translate a single "B" pixel by one pixel, each change contributes $q\Delta\Phi/(F_N/\tau) = 2\pi q/F_N$ to the additional phase in a staircase, which completes $q$ periods in one period of $\Phi$. We thus write the general phase term as a function of the modulation phase as

$$\theta_q(\Phi_i + \Delta\Phi) = \theta_q(\Phi_i) + q\Delta\Phi. \quad (6)$$

## S4-TOPOLOGICAL NUMBERS - STRUCTURAL ORIGIN

The purpose of this section is to provide a theoretical description of the experiment reported in Fig. 3 of the main article, *i.e.* to obtain the $(k_x, k_\Phi)$ map. We first recall basic results of the well-known "Cut and Project" construction of 1D quasicrystals, as well as recent results obtained in [1] that will be useful for the following. Then, we describe the global properties of the set $\{S_N(\Phi)\}$ of all possible Fibonacci chains of length $F_N$. This set corresponds to the pattern programmed on the DMD, and possesses specific geometrical and topological properties that we unveil. Finally, using these properties, we explain the observed diffraction pattern and describe it in terms of topological numbers.

### Finite-size Fibonacci chains. Role of the phason

The "Cut and Project" (C&P) method generates a quasiperiodic chain from a primitive $\mathbb{Z}^2$-lattice cut by a line $\Delta$ defined by $v = u\tan\theta + \text{const}$ (see Fig. 3a). We denote by $\Delta_\perp$ the direction perpendicular to $\Delta$ and define an acceptance window as a band of width $\Omega$ centered at $\Delta$. This realizes the "cut". A C&P set is obtained by projecting the $\mathbb{Z}^2$ points inside $\Omega$ on $\Delta$ and along $\Delta_\perp$. There are only two possible distances along $\Delta$ between neighboring projections, denoted $\{A, B\}$. One can generate the infinite Fibonacci chain $S_\infty$ by choosing $\tan\theta = \tau^{-1}$, $\tau$ being the golden mean. The choice of an origin on $\Delta$ is irrelevant for the infinite chain $S_\infty$, but not for finite chains $S_N$ of length $F_N$: the origin fixes the first letter and the iteration of the sequence. We note that C&P and characteristic function methods, as used in the main text, are related through the constant term in the equation for $\Delta$, namely $v = u\tan\theta - \frac{\Phi}{2\pi}$.

The C&P method allows to interpret the $2\pi$-periodic, structural degree of freedom $\Phi$ as the parameter driving the rearrangement of letters along the Fibonacci chain (see Fig. 3). For a chain of length $F_N$, each value of $\Phi$ generates a different segment of $S_\infty$, and corresponds to some translation along $\Delta$. Monitoring the phason $\Phi$ induces a series of $F_N$ identical local structural changes equivalent to the inversion of a single 6-letter string $BAABAB \leftrightarrow BABAAB$. These changes occur one at a time and are distributed according to a geometrical pattern (see Fig. 3c). The $\Phi$-axis, corresponding to the phason direction, is infinite. However, since $\Phi$ is $2\pi$-periodic, the structural information in the phason direction is contained in a single period.

To generate a *finite* chain $S_N$ of $F_N$ letters, the slope of the cut $\Delta$ defined by $\tan\theta$ must not necessarily be taken as an irrational number, but may be given by a rational approximant $p/q$ (as long as the unit cell of the resultant periodic chain remains larger than $F_N$). For

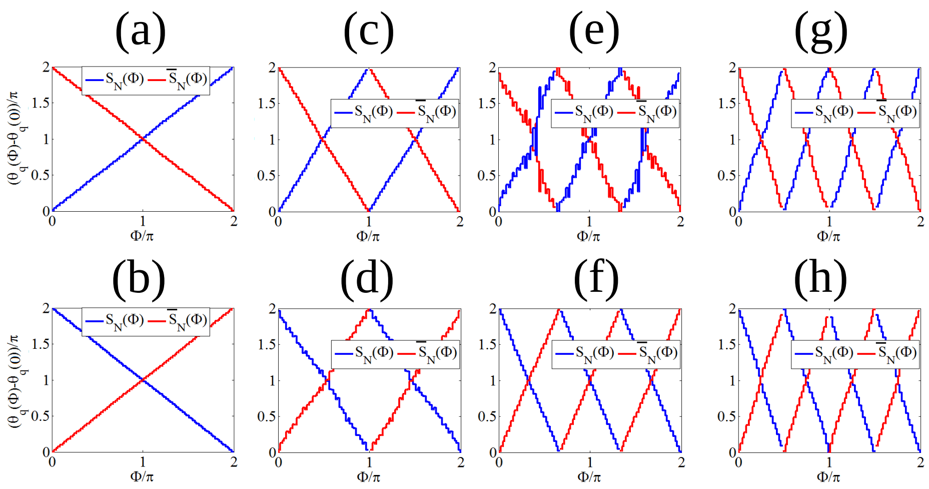

FIG. 2. A numerical plot of the phase $\theta_q(\Phi)$ of the diffraction amplitude, as a function of $\Phi$ for the structures $S_N$ (in blue) and $\overline{S}_N$ (in red) and for the diffraction peaks $k_q$ for various $q$. (a)-(b) $q=\pm1$, respectively. (c)-(d) $q=\pm2$, respectively. (e)-(f) $q=\pm3$, respectively. (g)-(h) $q=\pm4$, respectively.

.

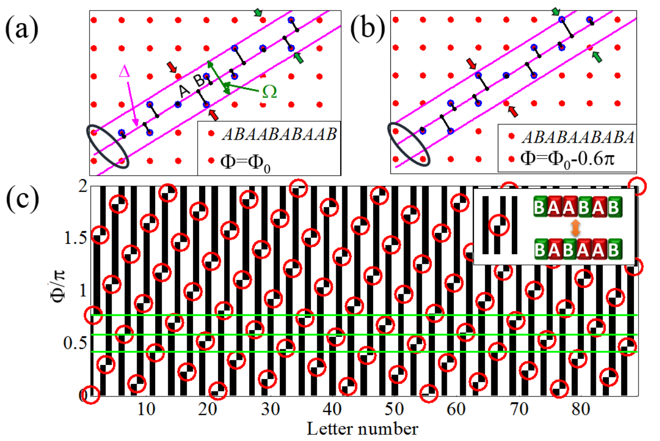

FIG. 3. Phason driving in the Cut & Project method for the slope $\tau^{-1}$. (a)-(b) The C&P method for the $\Phi$ values $\Phi_0$ and $\Phi_0-0.6\pi$. An ellipse indicates the origin of the chain. The 10 first letters of the resulting sequences are in the insets. Shifting the band $\Omega$ along the vertical axis induces two structural changes corresponding to points entering and leaving $\Omega$ (red/green arrows). (c) Structural color plot. Black(white) regions describe $B(A)$ letters. Identical structural changes (red circles, inset) occur when scanning $\Phi$ (e.g. green lines).

the "standard" Fibonacci chain of length 89 (obtained for instance with the substitution rule) $S_{10}(\Phi_{\rm std})$, the approximant has to be at least as good as 34/55. Similarly, to generate the complete set of $F_N$ finite chains, $S_N(\Phi)$, the slope can again be taken as another rational approximant $p/q$ (provided the unit cell of the resulting periodic pattern is larger than $2F_N+1$). For the set $\{S_{10}(\Phi)\}$ the approximant with the smallest possible $p$ is 89/144.

The C&P method also allows to obtain the Bragg peak structure of $S_\infty$ [6, 7]. In the case of a finite segment $S_N$, we have observed experimentally that there still exist diffraction peaks, located at approximate values of the exact Bragg peaks spatial frequencies, and also that we were able to probe their topological properties by scanning through the $F_N$ possible realizations (see Fig. 2 in the main text).

### Properties of the 2D set of Fibonacci chains $\{S_N(\Phi)\}$

We now consider the pattern described in Fig. 3c that is programmed on the DMD and whose diffraction pattern is the topological map of Fig. 3 in the main text. This finite 2D structure may be described as another $\mathbb{Z}^2$-lattice rotated by an angle $\varphi$ with respect to the $(x,\Phi)$ axes (see Fig. 4a).

Disregarding the form factor of the 2D unit cell of this structure, the remaining square lattice of points is represented by the function,

$$Q(x,\Phi)=\frac{1}{4\pi^2}\sum_{k,l}\delta(x-k\cos\varphi-l\sin\varphi)\times\delta(\Phi+k\sin\varphi-l\cos\varphi), \qquad (7)$$

where the sum is over a finite set of integers $(k,l)$. The Fourier transform (disregarding the effect of the finite size of the system on the peaks width) of the rotated $(x,\Phi)$ $\mathbb{Z}^2$- lattice is also a $\mathbb{Z}^2$-lattice rotated with the angle $\varphi$ with respect to the reciprocal space $(k_x,k_\Phi)$, and

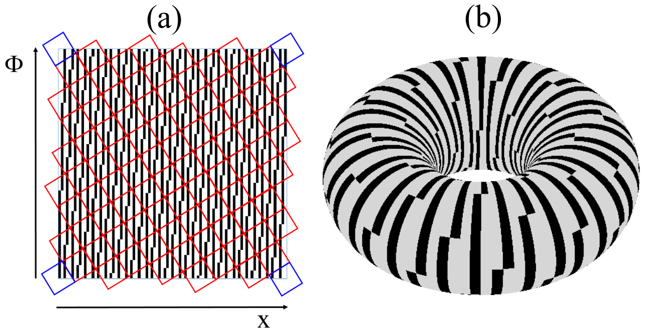


FIG. 4. Structural properties of the 2D set $\{S_N(\Phi)\}$ for $N = 10$. (a) The $\{S_N(\Phi)\}$ structural $x-\Phi$ map created through the Cut & Project method (see Fig. 3c) forms a tilted 2D crystal with a unit cell indicated by red and blue squares. This map is a torus obtained by wrapping the map along both axes, so that the four blue squares coincide. (b) An illustration of the resulting torus.

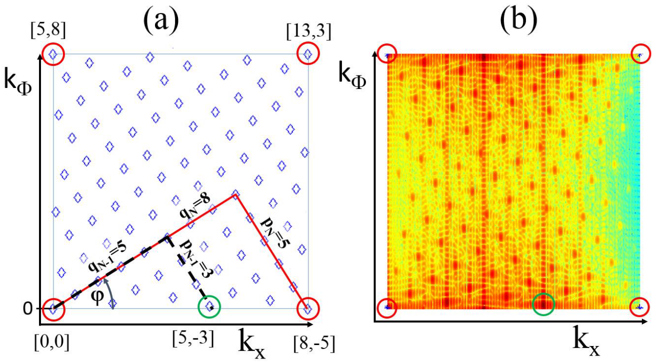


FIG. 5. Construction of the torus $\mathrm{QBZ}_N$ for $N = 10$ with the corresponding values $p_N = 5$ and $q_N = 8$. The red circles define the corners of the torus $\mathrm{QBZ}_N$ which encloses $F_{10} = 89$ points (lattice coordinates $[m, n]$ are given). The fundamental $k_\Phi$ value, $\delta k_\Phi$ corresponding to topological number equal to 1, is represented by the green circle. This lowest non zero value of $k_\Phi$ is obtained using the previous approximant $(p_{N-1}, q_{N-1})$ in the Farey series. (a) An emulated lattice angled at $\varphi$ (to set notations). (b) The actual 2D Fourier transform of $\{S_N(\Phi)\}$ for $N = 10$.

represented by,

$$F(k_x, k_\Phi) = \sum_{n,m} \delta(k_x - m\cos\varphi + n\sin\varphi) \times \delta(k_\Phi - m\sin\varphi - n\cos\varphi), \tag{8}$$

where the sum is over an infinite set of integers $(m, n)$. It is important to note that the rotation angle $\varphi$ is not given, for finite chains, by $\tan\varphi = \tau^{-1}$. For the set $\{S_N(\Phi)\}$ generated as discussed previously, the tiling angle of this new $\mathbb{Z}^2$- lattice has always a fixed rational slope

$$\tan\varphi = \frac{p_N}{q_N} \ , \tag{9}$$

where the two mutually prime integers $(p_N, q_N)$ depend only on $F_N$ [2]. For $S_{10}$, we have $p_N = 5$ and $q_N = 8$.

The $2\pi$-periodicity of the set $\{S_N(\Phi)\}$ in the phason direction $\Phi$, together with the fixed rational angle of rotation $\varphi$, means that the set may be folded to form a perfect torus (see Fig. 4b).

### Diffraction pattern in terms of topological numbers

We now discuss the diffraction pattern of the 2D structure of Fig. 3 to obtain both the (approximate) $k$ values of the Bragg peaks and the corresponding observable (exact) topological numbers.

The infinite reciprocal space of the finite set $\{S_N(\Phi)\}$ may be characterized by a finite quasi-Brillouin zone, $\mathrm{QBZ}_N$, (also a torus) which generalizes the usual notion of Brillouin zone. We use the fact that the rotation angle of the $\mathbb{Z}^2$ reciprocal lattice with respect to the $(k_x, k_\Phi)$ axes is still described by $\tan\varphi$ (see Fig. 5).

To build the torus $\mathrm{QBZ}_N$ in the $(k_x, k_\Phi)$ reciprocal space, we set an origin $(k_x, k_\Phi) = (0, 0)$ at some point and label them with the lattice coordinates $[m = 0, n = 0]$. The next step is to identify the three other corners of the $\mathrm{QBZ}_N$, using Eq. (9), to be $[m = q_N, n = -p_N]$ where $(k_x, k_\Phi) = (q_N\cos\varphi + p_N\sin\varphi, 0)$, $[m = p_N, n = q_N]$ where $(k_x, k_\Phi) = (0, p_N\sin\varphi + q_N\cos\varphi)$, and $[m = q_N + p_N, n = q_N - p_N]$ where $(k_x, k_\Phi) = (p_N\sin\varphi + q_N\cos\varphi, p_N\sin\varphi + q_N\cos\varphi)$. These four points define the torus $\mathrm{QBZ}_N$ as represented on Fig. 5. It exactly encloses $F_N$ points.

We now discuss the normalization of the reciprocal space torus coordinates. The $k_x$ coordinates may be normalized by $(p_N\sin\varphi + q_N\cos\varphi)^{-1} = 1/\sqrt{p_N^2 + q_N^2}$ so that $k_x \in [0, 1]$. After this normalization, the $F_N$ points at which $F(k_x, k_\Phi) \neq 0$ correspond to all possible (approximate) Bragg peaks values $k_q$. As for normalization along the $\Phi$-axis, it is obtained from the reciprocal lattice point $(\delta k_x, \delta k_\Phi)$ with $\delta k_\Phi$ the smallest nonzero value of $k_\Phi$. The (toroidal) vector between the origin and this lattice point is instrumental to find all points within the $\mathrm{QBZ}_N$ torus, namely through the recurrent addition (and winding) of this vector (see Fig. 5). This single fundamental lattice point is defined by $[m = q_{N-1}, n = -p_{N-1}]$, where $p_{N-1}$ and $q_{N-1}$ are obtained using the preceding approximant of the slope $\tan\varphi = p_N/q_N$ in the Farey sequence [2],

$$\frac{1}{1} : \frac{1}{1} : \frac{1}{2} : \frac{2}{3} : \frac{3}{5} : \frac{5}{8} : \cdots : \frac{p_j}{q_j} : \cdots \ . \tag{10}$$

In reciprocal space coordinates, we have

$$(\delta k_x, \delta k_\Phi) = \left( \frac{q_{N-1}\cos\varphi + p_{N-1}\sin\varphi}{\sqrt{p_N^2+q_N^2}}, \right. \\ \left. q_{N-1}\sin\varphi - p_{N-1}\cos\varphi \right). \quad (11)$$

The expression of $(\delta k_x, \delta k_\Phi)$ corresponds to the conumbering method developed in [8] and we use it to set the $k_\Phi$-scales in the reciprocal lattice. The normalized $k_\Phi$ coordinates correspond to the integer (topological) numbers

$$C(n,m) \equiv \frac{k_\Phi}{\delta k_\Phi} = \frac{m\sin\varphi + n\cos\varphi}{q_{N-1}\sin\varphi - p_{N-1}\cos\varphi} = mp_N + nq_N. \quad (12)$$

These topological numbers describe how many times the phase of the diffraction amplitude winds around the torus when scanning over a period in the $k_\Phi$ direction. The last equality is obtained by noting that successive approximants in the Farey series in Eq. (10) fulfill $|p_{N-1}q_N - q_{N-1}p_N| = 1$.

The Fourier transform in Eq. (8) can be rewritten in terms of the topological numbers $C$ and of the (approximate) Bragg peak values $k_x$ as,

$$F(k_x, C) = \sum_{n,m} \delta\left(k_x - \frac{m\cos\varphi - n\sin\varphi}{\sqrt{p_N^2+q_N^2}}\right) \\ \times\delta(C - mp_N - nq_N), \quad (13)$$

where the integers $(n,m)$ run over the torus $\mathrm{QBZ}_N$ now entirely defined by

$$k_x(m,n) = (mq_N - np_N)/(p_N^2+q_N^2), \\ C(m,n) = mp_N + nq_N. \quad (14)$$

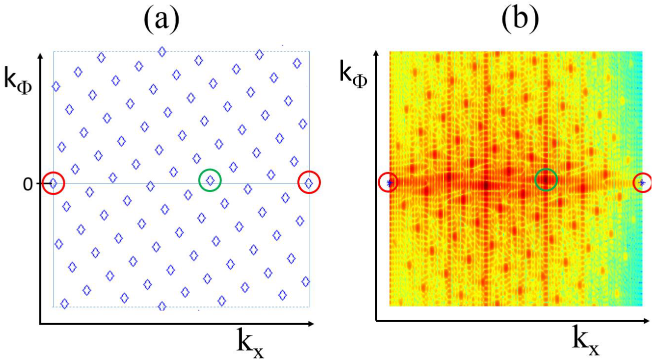


FIG. 6. A properly unwrapped torus $\mathrm{QBZ}_N$ for $N = 10$. The red circles define the 4 corners of the torus $\mathrm{QBZ}_N$ of Fig. 5. The fundamental $k_\Phi$ value, $\delta k_\Phi$ corresponding to topological number equal to 1, is represented by the green circle. $k_\Phi$ values now come in pairs of equal magnitude and opposite sign. (a) An emulated lattice angled at $\varphi$. (b) The actual 2D Fourier transform of $\{S_N(\Phi)\}$ for $N = 10$.

Additionally, a change of origin can be performed in the $k_\Phi$ toroidal dimension, such that all reciprocal lattice points with $F_N/2 \leq k_\Phi/\delta k_\Phi$ are wrapped around the torus to have $k_\Phi/\delta k_\Phi \to F_N/2 - k_\Phi/\delta k_\Phi$. The total number of points in the 2D torus $\mathrm{QBZ}_N$ is the number of topological integers available for a given $N$. It is given by $F_N$ and we have $|C(m,n)| \leq F_N/2$.

Finally, we note that topological numbers always appear in pairs of opposite sign associated to the structure length $F_N$ and its minimal Farey approximate $\tan(\theta) = p/q$. For the lowest approximant (periodic system), the values $C = \pm1$ will show up first, followed by higher paired values while increasing the ratio $p/q$. It is worth noting again that while the topological numbers $C(m,n)$ are always integers, the (approximate) Bragg vectors $k_x(m,n)$ depend on the chain length but they rapidly converge to the exact Bragg value obtained for $N \to \infty$.

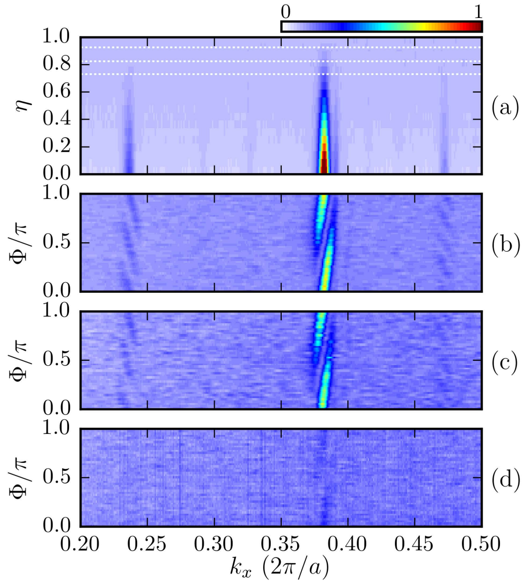


FIG. 7. Robustness of the topological features against structural noise. (a) Diffraction pattern of the Fibonacci and reversed Fibonacci chain at $\Phi = 0$ and for different levels of noise $\eta$. The white dotted lines correspond to three chosen examples. (b)-(d)Evolution of the diffraction pattern when varying $\Phi$ for different noise levels. (b) $\eta = 0.73$, (c) $\eta = 0.83$, (d) $\eta = 0.93$.

## S5-COMPLEMENTARY DATA: ROBUSTNESS AGAINST NOISE

In this section we present complementary measurements quantifying the influence on the diffraction signal of a controlled amount of noise on the DMD pattern. This study is performed with the configuration described in Fig. 2 of the main text.

We introduced noise in the following way. The initial

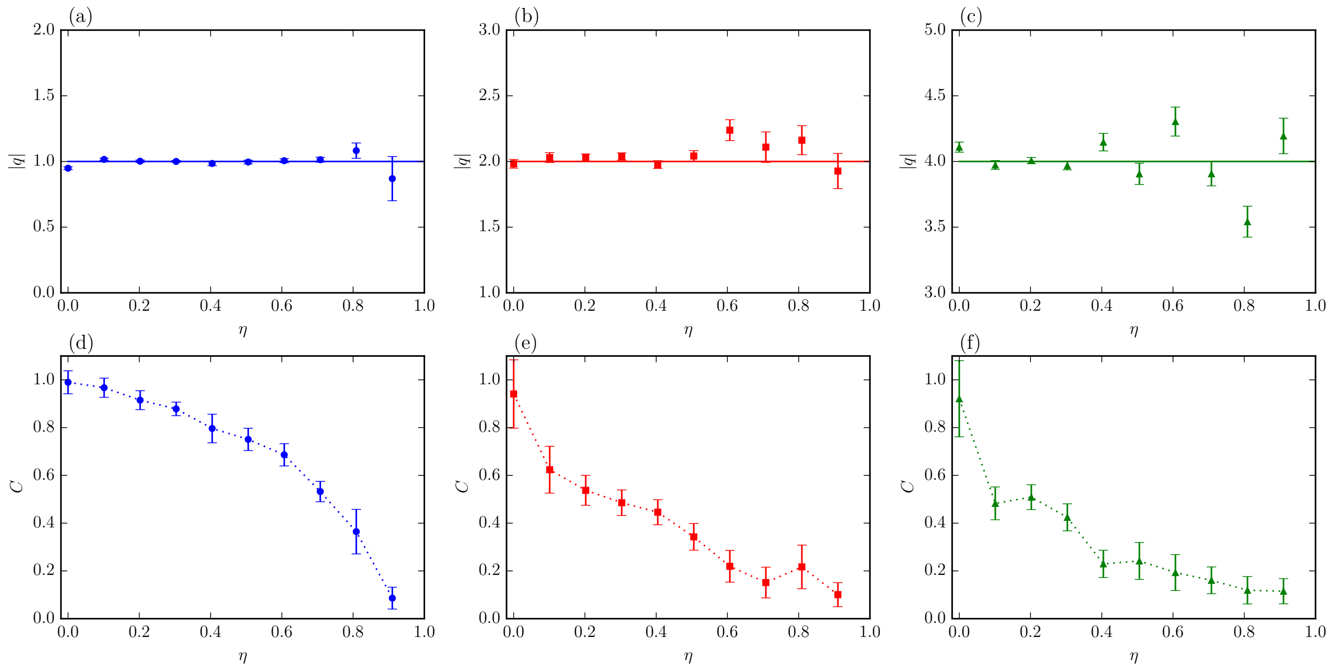


FIG. 8. Influence of noise on the $S_n + \overline{S}_n$ configuration for $q = 1$, $q = 2$ and $q = -4$. For each value of $q$ we record from the experimental image the signal on the pixel corresponding to the associated value of $k_x$. We repeat this procedure for each value of $\Phi$ and obtain the diffraction peak amplitude variation with $\Phi$. We fit the oscillations of the amplitude of the diffraction peaks when scanning $\Phi$ by $A + B\cos^2(q\Phi - \phi_s)$ at different amplitudes of the noise $\eta$. We show the values obtained for $|q|$ (a,b,c) and the corresponding contrast (d,e,f) of these oscillations defined by $C = B/(2A)$.The error bars correspond to the one standard deviation errors given by the fit algorithm. We observe that despite the strong decrease of the contrast the period stays constant.

.

signal is the Fibonacci chain with its mirrored image (see Fig. 2(c) in the main text). Noting $F_N$ the chain length (we used $F_N = 89$ in our experiments), the total signal has a length of $2F_N$. We randomly chose $N_{\rm noise}$ mirrors without replacement from the $2F_N$-long total chain. The state of the selected mirrors is then randomly chosen between reflective and non-reflective with equiprobability. The resulting one-dimensional chain is then replicated on each line of the DMD, so that the final pattern consists of a collection of vertical lines. This constitutes a single realization of a noisy pattern with a noise level $\eta = N_{\rm noise}/(2F_N)$. Note that this algorithm *a priori* generates independent noise for the two parts of the chain (Fibonacci and mirrored Fibonacci).

To average over several realizations of the noise pattern, we reproduced this procedure by randomly choosing a new set of mirrors and randomly flipping them. Each line from figures 7(a) to 7(d) is obtained by averaging the measured diffraction signal over 200 independent realizations of the noise. In order to speed up the data acquisition process, we dynamically control the DMD so that it scans over all the noise realizations during the CCD camera exposure time, and the average is made while the image is recorded.

We select in Fig. 7(b-d) three specific values of $\eta$ ($\eta = 0.73, 0.83$ and $0.93$) and show the evolution of the diffraction pattern when scanning $\Phi$. More quantitatively, we show in Fig. 8 the contrast of these oscillations and their period as a function of $\eta$ for $q = 1$, $q = 2$ and $q = -4$. Whereas the contrast of the oscillations decreases for an increasing noise level, we observe that the period is constant within statistical uncertainty due to imaging noise. This result illustrates the robustness against noise of the oscillation period.


[1] E. Levy, A. Barak, A. Fisher, and E. Akkermans, arXiv:1509.04028 (2015).
[2] E. Levy, et al., in preparation (2017).
[3] A. König and N. Mermin, Phys. Rev. B **56**, 13607 (1997).
[4] A. König and N. Mermin, Am. J. of Phys. **68**, 525 (2000).
[5] S. Parameswaran, A. Turner, D. Arovas, and A. Vishwanath, Nat. Phys. **9**, 299 (2013).
[6] V. Elser, Acta Cryst. **A42**, 36 (1986).
[7] R. Zia and W. Dallas, J. Phys. A **18**, L341 (1985).
[8] R. Mosseri and F. Bailly, Journal de Physique I **2**, 1715 (1992).
